# Supplementary material for: Findings of the NLP4IF-2021 Shared Tasks on Fighting the COVID-19 Infodemic and Censorship Detection
Source: arXiv:2109.12986 source file (2021-09-23)
Supplement: Supplementary file 1 [file appendix.tex]

\appendix

\section{Summary of all Systems Submitted to the COVID-19 Shared Task}\label{sec:systemsummary}

\textbf{DamascusTeam} \cite{NLP4IF-2021-DamascusTeam} 
used an approach based on the AraBERT model. It is in the form of a two-step pipeline, where the first step involves a series of pre-processing procedures to transform Twitter jargon, including emojis and emoticons, into plain text. In the second step a version of AraBERT was exploited to fine-tune and classify the tweets. The system ranked 5th on the Arabic dataset.

\textbf{Team dunder\_mifflin}~\cite{NLP4IF-2021-DunderMifflinTeam}
built a multi-output model using task-wise multi-head attention for inter-task information aggregation. This was built on top of the Bidirectional Encoder Representations obtained from the RoBERTa Transformer. To tackle the small size of the dataset back-translation was used for data augmentation. The loss-function was weighted for each output, in accordance with the distribution of labels for that output. They were the runners-up in the English subtask with a mean F$_1$-score of 0.891 on the test set, without the use of any task-specific embeddings or ensembles. 

\textbf{Team HunterSpeechLab}~\cite{NLP4IF-2021-HunterSpeechLabTeam} participated in all three subtasks. 
It explored the cross-lingual generalization ability of multitask models trained from scratch (logistic regression, transformer encoder) and pre-trained models (English BERT, m-BERT) for deception detection. 

\textbf{Team iCompass}~\cite{NLP4IF-2021-iCompassTeam} 
used state-of-the-art contextualized text representation models that were fine-tuned for the down-stream task in hand. ARBERT, MARBERT,AraBERT, Arabic ALBERT  and BERT-base-arabic were used. According to the results, BERT-base-arabic had the highest F$_1$ score on the test set, 0.748.

\textbf{Team InfoMiner}~\cite{NLP4IF-2021-InfoMinerTeam}
participated in all three subtasks. They used pre-trained transformer models, specifically BERT base cased, RoBERTa base, BERT multilingual cased and AraBERT. They optimized the transformer models for each question separately and used undersampling to deal with the fact that the data is imbalanced. They achieved 4-th place in all the languages. 

\textbf{Team NARNIA}~\cite{NLP4IF-2021-NARNIATeam} 
 have experimented with a number of Deep Learning based models, including different word embeddings, such as Glove, ELMo, among others. BERTweet model achieved the best overall F$_1$-score of 0.881 and secured the third rank on the English subtask.

\textbf{Team R00}~\cite{NLP4IF-2021-R00Team}
had the best performing system for the Arabic subtask. It used an ensemble of neural networks combining a linear layer on top of one out of the following four pre-trained Arabic language models: AraBERT, Asafaya-BERT, ARBERT, MARBERT. 

\textbf{Team TOKOFOU}~\cite{NLP4IF-2021-TOKOFOUTeam} participated in the English subtask.  
It gathered a collection of 6 BERT-based language models trained in domains (e.g., Twitter and COVID-themed data), or fine-tuned on tasks similar to the shared task’s topic (e.g., hate speech and sarcasm detection). Every model was then fine-tuned on the shared task data, projecting a label from the sequence classification token for each of the 7 questions in parallel. After carrying out model selection on the basis of development set F$_1$ performance, the team cast the models into a majority based ensemble to counteract the small size of the dataset and ensure robustness.

In Tables \ref{tab:overview_task1_english}, \ref{tab:overview_task1_arabic} and \ref{tab:overview_task1_bulgarian}, we report the participant's system approaches for English, Arabic and Bulgarian, respectively. Across all languages, it appears that participants have used transformer-based models, either mono or multilingual models. In terms of models, SVM and logistic regression are used. Some studies also used ensemble and data augmentation. 

\begin{table}[h!]
\centering
\setlength{\tabcolsep}{1.2pt}    
\small
\scalebox{0.8}{
\begin{tabular}{l|ll|ll|ll|lll}
\toprule
\multicolumn{1}{c}{\textbf{Ranks Team~}} & \multicolumn{2}{c}{\textbf{Trans.}} & \multicolumn{2}{c}{\textbf{Models}} & \multicolumn{2}{c}{\textbf{Repres.}} & \multicolumn{3}{c}{\textbf{Misc}} \\ \midrule
\textbf{~} & \rotatebox{90}{\textbf{BERT}} & \rotatebox{90}{\textbf{RoBERTa}} & \rotatebox{90}{\textbf{Logistic Regression}} & \rotatebox{90}{\textbf{SVM}} & \rotatebox{90}{\textbf{ELMo}} & \rotatebox{90}{\textbf{Golve}} & \rotatebox{90}{\textbf{Ensemble}} & \rotatebox{90}{\textbf{Under/over-sampling}} & \rotatebox{90}{\textbf{Data augmentation}} \\ \midrule
1. TOKOFOU & \sq & ~ & ~ & ~ & ~ & ~ & \sq & \multicolumn{1}{c}{~} & ~ \\
2. dunder\_mifflin & ~ & \sq & ~ & ~ & ~ & ~ & ~ & ~ & \sq \\
3. NARNIA & \sq & ~ & ~ & \cq & \cq & \cq & \cq & ~ & ~ \\
4. InfoMiner & \sq & \cq & ~ & ~ & ~ & ~ & ~ & \sq & ~ \\
7. HunterSpeechLab & \sq & ~ & \sq & ~ & ~ & ~ & ~ & ~ & ~ \\ \bottomrule
\end{tabular}
}

\setlength{\tabcolsep}{1.2pt}
\begin{tabular}{@{}rl@{}}
1 & \cite{NLP4IF-2021-TOKOFOUTeam} \\
2 & \cite{NLP4IF-2021-DunderMifflinTeam} \\
3 & \cite{NLP4IF-2021-NARNIATeam} \\
4 & \cite{NLP4IF-2021-InfoMinerTeam} \\
7 &  \cite{NLP4IF-2021-HunterSpeechLabTeam} 
\end{tabular}

\caption{Task 1: Overview of the approaches used by the participating systems for \textbf{English}. \sq$=$part of the official submission; \cq$=$considered in internal experiments; \emph{Trans.} is for Transformers; \emph{Repres.} is for Representations. References to system description papers are shown below the table.
}
\label{tab:overview_task1_english}
\end{table}

\begin{table}[h!]
\centering
\setlength{\tabcolsep}{1.2pt}    
\small
\scalebox{0.8}{
\begin{tabular}{l|llllll|l|ll}
\toprule
\multicolumn{1}{c}{\textbf{Ranks Team}} & \multicolumn{6}{c}{\textbf{Trans.}} & \multicolumn{1}{c}{\textbf{Models}} & \multicolumn{2}{c}{\textbf{Misc}} \\ \midrule
\textbf{~} & \begin{sideways}\textbf{BERT multilingual}\end{sideways} & \begin{sideways}\textbf{AraBERT}\end{sideways} & \begin{sideways}\textbf{Asafaya-BERT}\end{sideways} & \begin{sideways}\textbf{ARBERT}\end{sideways} & \begin{sideways}\textbf{ALBERT}\end{sideways} & \begin{sideways}\textbf{MARBERT}\end{sideways} & \begin{sideways}\textbf{Logistic Regression}\end{sideways} & \begin{sideways}\textbf{Ensemble}\end{sideways} & \begin{sideways}\textbf{Under/over-sampling}\end{sideways} \\ \midrule
1. R00 & ~ & \sq & \sq & \sq & ~ & \sq & ~ & \sq & ~ \\
* iCampass & ~ & \sq & ~ & \cq & \cq & \cq & ~ & ~ & ~ \\
2. HunterSpeechLab & \sq & ~ & ~ & ~ & ~ & ~ & \sq & ~ & ~ \\
4. InfoMiner & \cq & \sq & ~ & ~ & ~ & ~ & ~ & ~ & \sq \\
5. DamascusTeam & ~ & ~ & ~ & \sq & ~ & ~ & ~ & ~ & ~ \\ \bottomrule
\end{tabular}
}

\setlength{\tabcolsep}{1.2pt}
\begin{tabular}{@{}rl@{}}
1 & \cite{NLP4IF-2021-R00Team} \\
$*$ & \cite{NLP4IF-2021-iCompassTeam} \\
2 & \cite{NLP4IF-2021-HunterSpeechLabTeam} \\
4 & \cite{NLP4IF-2021-InfoMinerTeam} \\
5 &  \cite{NLP4IF-2021-DamascusTeam} 
\end{tabular}

\caption{Task 1: Overview of the approaches used by the participating systems for \textbf{Arabic}. \sq$=$part of the official submission; \cq$=$considered in internal experiments; \emph{Trans.} is for Transformers; \emph{Repres.} is for Representations. References to system description papers are shown below the table.
}
\label{tab:overview_task1_arabic}
\end{table}

\begin{table}[h!]
\centering
\setlength{\tabcolsep}{1.2pt}    
\small
\scalebox{0.8}{
\begin{tabular}{l|l|l|l}
\toprule
\multicolumn{1}{c}{\textbf{Ranks Team~}} & \multicolumn{1}{c}{\textbf{Trans.}} & \multicolumn{1}{c}{\textbf{Models}} & \multicolumn{1}{c}{\textbf{Misc}} \\ \midrule
~ & \begin{sideways}\textbf{BERT multilingual}\end{sideways} & \begin{sideways}\textbf{Logistic Regression}\end{sideways} & \begin{sideways}\textbf{Under/over-sampling}\end{sideways} \\ \midrule
2. HunterSpeechLab & \sq & \sq & ~ \\
4. InfoMiner & \sq & ~ & \sq \\ \bottomrule
\end{tabular}
}

\setlength{\tabcolsep}{1.2pt}
\begin{tabular}{@{}rl@{}}
2 &  \cite{NLP4IF-2021-HunterSpeechLabTeam} \\
4 & \cite{NLP4IF-2021-InfoMinerTeam}
\end{tabular}
\caption{Tassk 1: Overview of the approaches used by the participating systems for \textbf{Bulgarian}. \sq$=$part of the official submission; \cq$=$considered in internal experiments; \emph{Trans.} is for Transformers; \emph{Repres.} is for Representations. References to system description papers are shown below the table.
}
\label{tab:overview_task1_bulgarian}
\end{table}
